# Supplementary material for: Corruption-Robust Offline Two-Player Zero-Sum Markov Games
Source: arXiv:2403.07933 source file (2024-03-04)
Supplement: Supplementary file 1 [file agnostic_result.tex]

\subsection{Proof of Theorem \ref{thm:agnostic_learning}}

We restate the result.
\begin{statement}
    For every algorithm $L$ that achieves a diminishing suboptimality gap in a clean environment, there exist linear Markov games $\mathcal{G}_1$ and $\mathcal{G}_2$, corruption model $C$, and a data collecting distribution $d^\rho$ such that, for every $\epsilon \in (0,1/2]$, $L$ achieves 
    \begin{equation*}
        \optgap (\widehat{\pi},\widehat{\nu}) \geq \Omega (1/2)~,
    \end{equation*}
    with probability at least $1/4$, in at least one of the games.
\end{statement}

\begin{proof}
    Let $N=KH$ and let $p\in (0,1)$. Let us construct two simple bandit instances, with action sets $\{ (a_1,b_1),(a_1,b_2),(a_2,b_1),(a_2,b_2)\}$, as follows. For game $\mathcal{G}_1$ we have 
    \begin{align*}
        r_1(a_1,b_1)= Ber (\frac{1}{2}+\frac{\epsilon}{4pN}), \;\; r_1(a_2,b_1)=Ber (\frac{1}{2}) \;\; \text{and} \;\; r_1(a_1,b_2)=r_1(a_2,b_2)=0~.
    \end{align*}
    Let the data-collecting distribution be such that $d^\rho(a_1,b_1) = d^\rho(a_1,b_2)= p/2$ and $d^\rho(a_2,b_1)=d^\rho(a_2,b_2)=(1-p)/2$. Note that the LRU constant here is $c_1=2/p$.
    
    Next, for game $\mathcal{G}_2$, we let
    \begin{align*}
         r_2(a_1,b_1)= Ber (\frac{1}{2}-\frac{\epsilon}{4pN}), \;\; r_2(a_2,b_1)=Ber (\frac{1}{2}) \;\; \text{and} \;\; r_2(a_1,b_2)=r_2(a_2,b_2)=0~.
    \end{align*}
    Let the data collecting distribution be the same as in $\mathcal{G}_1$. Here, we have that the LRU constant is $c_1=2/(1-p)$.

    Now let $D_1$ and $D_2$ be two datasets of size $N$ generated by the data-collecting distribution $d^\rho$ in compliance with $\mathcal{G}_1$ and $\mathcal{G}_2$, respectively. Note that $n(a_1,b_1):= n_1(a_1,b_1)=n_2(a_1,b_1)$, $n_1(a_1,b_2)=n_2(a_1,b_2)$, $n_1(a_2,b_1)=n_2(a_2,b_1)$ and $n_1(a_2,b_2)=n_2(a_2,b_2)$, where $n_1$ and $n_2$ count the occurrences of their arguments in $D_1$ and $D_2$, respectively. Also, the rewards $r_1(a_2,b_1)$ and $r_2(a_2,b_1)$ are sampled from $Ber(1/2)$, while $r_i(a_j,b_2)=0$, for $i,j\in \{ 1,2\}$. For the rest, let us consider the following construction. 

    Let $X_i$ and $Y_i$, for $i\geq 1$, be Bernoulli random variables defined as
    \begin{equation*}
        X_i = 
        \begin{cases}
            0 & \text{if} \;\; U \leq \frac{1}{2} - \frac{\epsilon}{4pN} \\
            1 & \text{otherwise}
        \end{cases}
        \;\; \text{and} \;\;
        Y_i =
        \begin{cases}
            0 & \text{if} \;\; U \leq \frac{1}{2} + \frac{\epsilon}{4pN} \\
            1 & \text{otherwise}
        \end{cases}
    \end{equation*}
    where $U$ is a uniform random variable in $[0,1]$. Then, $(X_i,Y_i)$ is a coupling with law 
    \begin{align*}
        \mathbb{P}\left( (X_i,Y_i)=(0,0) \right) & = \frac{1}{2} - \frac{\epsilon}{4pN}, \;\;\;\; \mathbb{P}\left( (X_i,Y_i)=(0,1) \right) = 0, \\ 
        \mathbb{P}\left( (X_i,Y_i)=(1,0) \right) & = \frac{\epsilon}{2pN}, \;\;\;\; \mathbb{P}\left( (X_i,Y_i)=(1,1) \right) = \frac{1}{2} - \frac{\epsilon}{4pN}.
    \end{align*}
    Now, let the rewards for $(a_1,b_1)$ be generated from $X_i$ and $Y_i$ in $\mathcal{G}_1$ and $\mathcal{G}_2$, respectively. We are interested in computing a lower bound on the probability that the rewards seen from $(a_1,b_1)$ in both datasets are indistinguishable.  To that end, we compute the following:
    \begin{align}
        \mathbb{P}\left( \sum^{n(a_1,b_1)}_{i=1} \mathbf{1}( X_i \neq Y_i) =0\right) & = \sum_{t\geq 1} \mathbb{P}\Bigl( n(a_1,b_1) = t \Bigr) \mathbb{P}\left(\sum^t_{i=1} \mathbf{1}(X_i\neq Y_i) =0\right) \label{eq:agnosticity_01}\\
                & \geq \mathbb{P}\Bigl( n(a_1,b_1) \leq pN \Bigr) \mathbb{P}\left(\sum^{pN}_{i=1} \mathbf{1}(X_i\neq Y_i) =0\right) \nonumber \\
                & = \frac{1}{2}  \left( 1 - \mathbb{P}\left( \sum^{pN}_{i=1} \mathbf{1}(X_i\neq Y_i) \neq 0\right) \right) \label{eq:agnosticity_02}\\
                & \geq \frac{1}{2}\left( 1- \sum^{pN}_{i=1}\mathbb{P}\left( X_i \neq Y_i \right) \right) \label{eq:agnosticity_03}\\
                & = \frac{1}{2} \left( 1 - pN \frac{\epsilon}{2pN}\right) \nonumber \\
                & \geq \frac{1}{4}~,\label{eq:agnosticity_04}
    \end{align}
    where \eqref{eq:agnosticity_01} follows from the law of total probability; \eqref{eq:agnosticity_02} follows from the fact that $n(a_1,b_1)$ is a Binomial random variable with mean $pN$; for \eqref{eq:agnosticity_03} we apply the union bound and \eqref{eq:agnosticity_04} follows from the fact that $\epsilon < 1$. 

    The above implies that, with probability at least $1/4$, the two games are indistinguishable. The adversary can replace $\epsilon N$ tuples $(a_1,b_1,0)$ with $(a_1,b_1,1)$ in $D_2$ to replicate $D_1$. Note that, no algorithm can be optimal in both settings, and will suffer a suboptimality gap of at least $\epsilon /2p$ in one of the games. As $p$ goes to $0$, the gap goes to $\infty$, while the constant $c_1$ remains bounded. This contradicts the statement of the theorem.
\end{proof}
