# Supplementary material for: Corruption-Robust Offline Two-Player Zero-Sum Markov Games
Source: arXiv:2403.07933 source file (2024-03-04)
Supplement: Supplementary file 2 [file appendix_algorithms.tex]

\section{Algorithm pseudocodes}\label{sec:algorithms}

\begin{algorithm}
\setstretch{1.2}
\caption{SCRAM-PMVI}
\label{alg:scram_PMVI}
\begin{algorithmic}[1]
\State \textbf{Input}: Dataset $D$, failure probability $\delta$, SCRAM.
\State \textbf{Initialize:} Randomly split dataset $D$ into $H$ subsets $D_h$ of cardinality $K$; set $\underline{V}_{H+1}(s_1)=\overline{V}_{H+1}(s_1)=0$.
\For{$h=H,H-1,\ldots,1$}:
% \State $\Lambda_h = \sum^K_{\tau=1}\phi^\tau_h(\phi^\tau_h)^\top + I$
\State Compute estimates $\underline{\omega}_h$ and $\overline{\omega}_h$ via SCRAM.
\State  $\underline{Q}_h(\cdot,\cdot,\cdot) \leftarrow \Pi_{H-h+1}\left( \phi(\cdot,\cdot,\cdot)^\top \underline{\omega}_h - \Gamma_h(\cdot,\cdot,\cdot) \right)$. \State $\overline{Q}_h(s,a,b)\leftarrow \Pi_{H-h+1}\left( \phi(\cdot,\cdot,\cdot)^\top \underline{\omega}_h + \Gamma_h(\cdot,\cdot,\cdot) \right)$.
\State Compute $(\widehat{\pi}_h, \nu'_h)$ and $(\pi'_h,\widehat{\nu}_h)$ as NE solutions to $\underline{Q}_h(\cdot, \cdot, \cdot)$ and $\overline{Q}_h(\cdot, \cdot, \cdot)$, respectively. 
\State  $\underline{V}_h(\cdot) \leftarrow \mathbb{E}_{a\sim \widehat{\pi}(\cdot |\cdot),b\sim \nu'(\cdot |\cdot)}[\underline{Q}_h(\cdot,a,b)]$. 
\State $\overline{V}_h(\cdot) \leftarrow \mathbb{E}_{a\sim \pi'(\cdot |\cdot),b\sim \widehat{\nu}(\cdot |\cdot)}[\overline{Q}_h(\cdot,a,b)]$.
\EndFor
\State \textbf{Output:} $\widehat{\pi} = (\widehat{\pi}_h)^H_{h=1},\widehat{\nu}=(\widehat{\nu}_h)^H_{h=1}$. 
\end{algorithmic}
\end{algorithm}

\begin{algorithm}
\setstretch{1.2}
\caption{Filtering PMVI}
\label{alg:filtering_PMVI}
\begin{algorithmic}[1]
\State \textbf{Input}: Dataset $D$, failure probability $\delta$, Filtering.
\State \textbf{Initialize:} Randomly split dataset $D$ into $H$ subsets $D_h$ of cardinality $K$; set $\underline{V}_{H+1}(s_1)=\overline{V}_{H+1}(s_1)=0$.
\For{$h=H,H-1,\ldots,1$}:
% \State $\Lambda_h = \sum^K_{\tau=1}\phi^\tau_h(\phi^\tau_h)^\top + I$
\State $(\widehat{r}_h, \widehat{p}_h ) \leftarrow \text{Filtering}(D_h, \epsilon)$.
\State Set $\underline{Q}_h(s,a,b)$ and $\overline{Q}_h(s,a,b)$ as in \eqref{eq:tabular_values_estimates_1} and \eqref{eq:tabular_values_estimates_2}.
\State Compute $(\widehat{\pi}_h, \nu'_h)$ and $(\pi'_h,\widehat{\nu}_h)$ as in Algorithm \ref{alg:scram_PMVI}.
\State Compute $\underline{V}_h(\cdot)$ and $\overline{V}_h(\cdot)$ as Algorithm \ref{alg:scram_PMVI}.
\EndFor
\State \textbf{Output:} $\widehat{\pi} = (\widehat{\pi}_h)^H_{h=1},\widehat{\nu}=(\widehat{\nu}_h)^H_{h=1}$. 
\end{algorithmic}
\end{algorithm}
